# Supplementary material for: Analysis of Collaboration in CS Prizewinning with a Nobel-Turing Comparison
Source: arXiv:2512.23919 ancillary file (2025-12-30)
Supplement: Supplementary file 1 [file SI.pdf]

# Supplementary Information for: Analysis of Collaboration in CS Prizewinning with a Nobel-Turing Comparison

Boleslaw K. Szymanski<sup>1\*</sup>, Yongtao Zhang<sup>2</sup>, Brian Uzzi<sup>3</sup>,  
Mohammed Shahid Modi<sup>1</sup>

<sup>1\*</sup>Department of Computer Science, Rensselaer Polytechnic Institute,  
110 8th St, Troy, 12180, NY, USA.

<sup>2</sup>Zhejiang University, 866 Yuhangtang Road, Hangzhou, 310058, China.

<sup>3</sup>Kellogg School of Management, Northwestern University, 2211  
Campus Dr, Evanston, 60208, IL, USA.

\*Corresponding author(s). E-mail(s): [szymab@rpi.edu](mailto:szymab@rpi.edu);  
Contributing authors: [yongtao.zhang@zju.edu.cn](mailto:yongtao.zhang@zju.edu.cn);  
[uzzi@northwestern.edu](mailto:uzzi@northwestern.edu); [modim2@rpi.edu](mailto:modim2@rpi.edu);

## S1 Data Description

We compile a comprehensive dataset of 105 recognized scientific prizes in computer science, awarded to 5,416 scholars through prizewinning events from 1965 to 2022. Our data sources include awards recorded by the Association for Computing Machinery (ACM), such as the prestigious Turing Award, ACM Fellow, and ACM Distinguished Members, and awards listed on Wikipedia’s pages for computer science awards. This dataset encompasses nearly all recorded scientific prizes in the computer science field, including traditional awards and contest awards like Olympiad medals, best paper awards at specific conferences, and so on. To ensure the robustness of our analysis, we only include prizes awarded to at least ten scientists. We link these prizes to scientists’

detailed research profiles using data from the SciSciNet dataset, which contains information on over 172 million publications by 209 million authors across 48,000 journals from 1800 to 2022.

Our methodology incorporates a fuzzy string-matching algorithm to accurately discern the identities of awardees within the SciSciNet dataset. This technique facilitates the reconciliation of variations in the spelling and formatting of prizewinners' names with those listed in SciSciNet.

We initially conducted preliminary filtering for cases involving multiple candidates sharing the same name. To disambiguate the winner, we exclude scholars whose first publication date is after the year the winners received the award and those who published papers within the last decade cited less than ten times. Given our focus on computer science prizewinners, as reflected in their publications, the winners have significantly contributed to their fields. Therefore, we also calculate the number of papers for each candidate classified under computer science. Among the candidates remaining after preliminary filtering, we presume that the one with the highest number of publications in computer science is the actual awardee.

We undertake a rigorous cross-validation exercise to validate the efficacy of our matching procedure. We randomly selected a subset of 100 awardees for manual verification to create the accuracy benchmark by comparing their identities and the corresponding SciSciNet authors' indices against our algorithmic matches.

We also conducted an approach using the large language model GPT-4. We augmented our identification process for homonymous scholars by gathering the titles of the first three most-cited papers associated with each name. Then, for each winner selected manually, we input the name of the award and the recipient, the year the recipient received the award, the recipient's region, and the titles of their highly cited papers into GPT-4. Then, we used customized prompts to discern the actual recipient among the candidates. Two cross-validation experiments showed that our matching strategy achieves a precision rate of approximately 92%, demonstrating our approach's robustness.

## S2 Prize Transition Matrix

We employ a heatmap to visualize this conditional probability adjacency matrix to show the dynamic relationship among different prizes. As depicted in Fig. S1a, across various pairs of prizes, some positions in the matrix exhibit a value  $A_{ij}$  that reaches 25,000, indicating that collaborators of the winners of prize  $i$  are 25,000 times more likely to win prize  $j$  compared to the baseline probability. Conversely, some entries

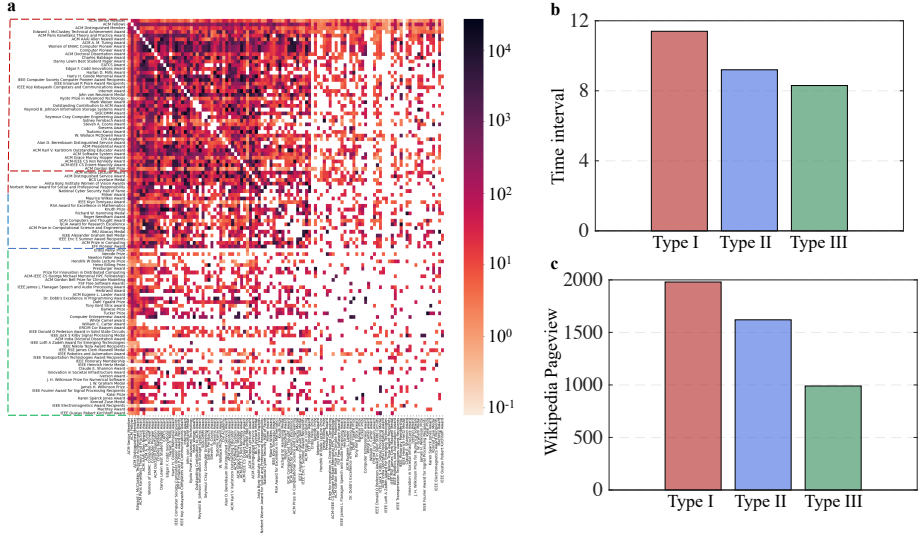

**Fig. S1: Scientific prize transition matrix.** **a**, Heatmap displays the values of  $A_{ij}$  of the matrix devised in Eq. 1 (main paper) on a logarithmic scale. Each cell in the map represents the ratio of the conditional probability of winning prize  $j$  given collaboration with the winners of prize  $i$  to the unconditional probability of winning prize  $j$ . The x-axis represents prize  $i$ , and the y-axis represents prize  $j$ . The white background corresponds to a value of 0. **b**, Career age of prizewinners, quantified by the time interval from their first publication to prizewinning, shows that winners of the first type of prizes typically have longer careers before winning, indicating they are at a later career stage. **(c)** Public notability of three different types of prizes, quantified by average Wikipedia page views from 2013 to 2023.

where  $A_{ij} = 0$  indicate that no collaborators of the winners of prize  $i$  have ever won prize  $j$ . We divided the prizes into three groups based on the distribution of color blocks in the heatmap. The first type of prize has a close relationship with each other, primarily reflected in the higher likelihood of winning these prizes for individuals who have collaborated with previous awardees. These prizes mainly focus on high-level, lifetime achievements and distinguished contributions.

The second type of prize shows less internal correlation than the first type. However, collaboration with awardees of the first type of prize still significantly increases the likelihood of winning these second-type prizes. The third type of prize exhibits minimal internal cooperation; such collaboration provides merely a slight advantage in winning these awards. This category emphasizes various technical achievements and innovations across multiple sub-fields. Compared to the first and second types, prizes of the third type focus more on specific sub-disciplines and narrower areas, such as

**Table S1:** Summary Statistics of Author Covariates by Objective and Prize-Winning Status

| Objective    | Group        | Degree              | Pub Count          | Avg Citations     | Career Span      | Avg Disruption   |
|--------------|--------------|---------------------|--------------------|-------------------|------------------|------------------|
| Whole-Career | Prizewinners | 275.04<br>(1535.28) | 154.44<br>(206.59) | 44.43<br>(93.35)  | 27.66<br>(16.32) | 0.007<br>(0.031) |
|              | Non-winners  | 789.98<br>(2759.44) | 45.00<br>(115.89)  | 52.08<br>(309.74) | 9.03<br>(12.40)  | 0.004<br>(0.038) |
| Pre-Award    | Prizewinners | 141.66<br>(811.97)  | 93.31<br>(132.96)  | 68.65<br>(221.94) | 20.86<br>(13.89) | 0.010<br>(0.041) |
|              | Non-winners  | 685.73<br>(2219.84) | 32.47<br>(84.50)   | 75.22<br>(384.59) | 9.96 (9.51)      | 0.005<br>(0.041) |

Values are presented as Mean (Standard Deviation).

signal processing, electromagnetic, and numerical software. Fig. S1b shows the career age of prize winners, quantified by the time interval between the year they publish the first paper and the year of prizewinning. As seen in the figure, winners of the first type of prize require more effort and time before winning, indicating a more significant time gap. The second type of prize has a smaller time gap, while the third type has the smallest. This implies that winners of the first type of prize are generally later in their academic careers than recipients of the other two types.

To further investigate the differences among these three groups of prizes, we examine their public notability. Public notability refers to the degree of public attention a prize receives. A higher notability score indicates greater importance, as it garners more attention from the public. We use Wikipedia Pageviews as a metric to measure public notability, obtained from the Wikipedia Pageviews API. To account for yearly fluctuations in pageview numbers, we calculate the average pageview over the last 10 years (2013-2023) as the public notability for each prize. As shown in Fig. S1c, the first type of prize has the highest average pageview, followed by the second and third types. These differences indicate that prizes for lifetime achievements receive more public attention than others, while prizes focusing on specific sub-disciplines and narrower areas are relatively less critical.

### S3 Covariate Analysis and Model Results for CEM

The attributes used for our analysis of prizewinning probabilities based on strong collaboration, their averages and standard deviations for prizewinners and non-winners are shown in Table S1. We considered the idea of a 'strong' collaboration in different ways, such as the number of papers co-authored by the prizewinner-author pair, total

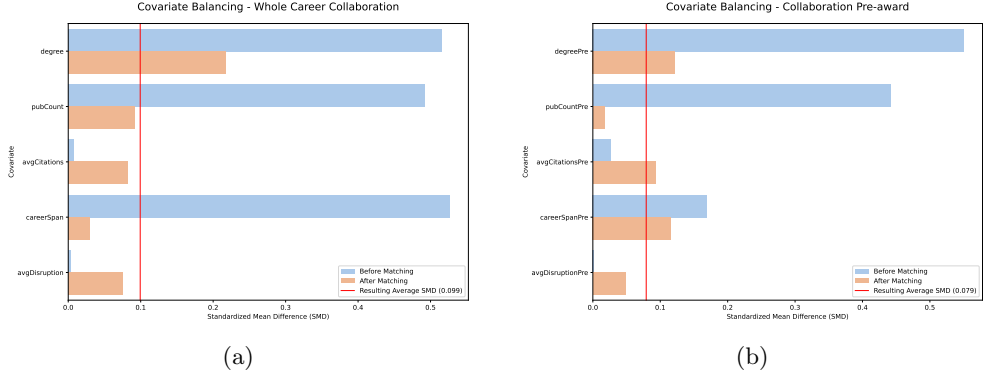

**Fig. S2:** Matching quality before and after coarsening each covariate. **(A)** is for the Whole-career collaboration objective, while **(B)** is for the pre-award collaboration objective. The preferred SMD for any covariate is  $< 0.1$ , and we consider an average SMD under that value to be indicative of sufficiently similar groupings.

citations received across all their papers or a combination of both those attributes. For both objectives, the best matching outcome was when we used the number of co-authored papers to represent collaboration strength.

### S3.1 Balance Matching and ATE of Matched Samples

We bin the authors into four groups based on the number of shared papers they have with a prizewinner, with those in the top two groups considered the treatment groups and the bottom two being the control. For the whole-career collaboration objective, this is straightforward as every author has some number of co-authored papers with a prizewinner. In case an author is connected to multiple prizewinners, the relationship with the highest number of co-authored papers between the pair is chosen. After this, we calculate the average SMD before matching as 0.3154 which is imbalanced.

For authors in the pre-award collaboration objective, the number of papers they have co-authored with a prizewinner is determinable only if they eventually win their own prize. For such authors, we find that the average number of years of collaboration with a prizewinner prior to winning their own award is between 3-4 years. For the remaining authors (non-winners), we calculate the number of co-authored papers they have in the first five years of collaboration with the prizewinners they co-authored with. Thus, for both winners and non-winners, the co-authored papers number for this objective represents their early relationship with a prizewinner and we use this to bin the authors into treatment and control groups similar to before and also compute

**Table S2:** Logistic Regression Results for Whole-Career Collaboration

| Variable                                | Odds Ratio | 95% CI                | P-value           |
|-----------------------------------------|------------|-----------------------|-------------------|
| <b>Strong Collaboration (T)</b>         | 3.950      | <b>[3.548, 4.396]</b> | <b>&lt; 0.001</b> |
| <i>Control Variables (Standardized)</i> |            |                       |                   |
| Degree                                  | 0.183      | [0.150, 0.223]        | < 0.001           |
| Publication Count                       | 1.523      | [1.464, 1.586]        | < 0.001           |
| Career Span                             | 1.511      | [1.467, 1.556]        | < 0.001           |
| Average Disruption                      | 1.078      | [1.040, 1.117]        | < 0.001           |
| Average Citations                       | 0.945      | [0.872, 1.023]        | 0.164             |
| <i>Model Summary</i>                    |            |                       |                   |
| Observations                            | 212,111    |                       |                   |
| Pseudo R-squ. (CS)                      | 0.011      |                       |                   |

**Note:** Table displays odds ratios from a weighted logistic regression model. The dependent variable is whether an author won a prize (1/0). The treatment (Strong Collaboration) is the number of co-authored papers with a prizewinner over whole career. Control variables were standardized before inclusion in the model.

the attributes with same rationale. The average SMD before matching in this case is 0.2405 which we consider imbalanced.

After forming treatment and control groups, we use a greedy balancing algorithm that iteratively coarsens each of the five covariates into a number of bins with eleven possible choices ([2, 3, 4, 5, 6, 7, 8, 16, 32, 64, 128]) until the best number of bins to minimize SMD for that covariate is found. Once this process finishes for all five covariates, the average SMD is calculated. This process leads to many observations being pruned, with 22% of the authors being retained in the matched strata for the whole-career collaboration objective and 12.6% of them being retained for the pre-award collaboration objective. The process effectively lowers the average SMD below the threshold, with degree (number of co-authors) being the only covariate that remains imbalanced for the first objective, and with degree and career span being slightly imbalanced for the second objective. While it may be possible to balance these attributes better, this would lead to more observations being pruned which is the tradeoff. The exact values of SMD before and after matching along with the final average SMD is visualized in Figure S2 for both objectives.

### S3.2 Model Outcomes

The exact odds ratios, confidence intervals and P-values for the pre-award and whole-career objectives are shown in Tables S3 and S2 respectively.

**Table S3:** Logistic Regression Results for Pre-Award Collaboration

| Variable                                | Odds Ratio | 95% CI                | P-value           |
|-----------------------------------------|------------|-----------------------|-------------------|
| <b>Strong Collaboration (T)</b>         | 5.997      | <b>[5.188, 6.932]</b> | <b>&lt; 0.001</b> |
| <i>Control Variables (Standardized)</i> |            |                       |                   |
| Degree                                  | 0.019      | [0.012, 0.029]        | < 0.001           |
| Publication Count                       | 2.292      | [2.126, 2.471]        | < 0.001           |
| Career Span                             | 1.543      | [1.487, 1.602]        | < 0.001           |
| Average Disruption                      | 1.157      | [1.118, 1.197]        | < 0.001           |
| Average Citations                       | 1.046      | [0.984, 1.112]        | 0.151             |
| <i>Model Summary</i>                    |            |                       |                   |
| Observations                            | 121,579    |                       |                   |
| Pseudo R-squ. (CS)                      | 0.018      |                       |                   |

**Note:** Table displays odds ratios from a weighted logistic regression model. The dependent variable is whether an author won a prize (1/0). The treatment (Strong Collaboration) is based on pre-award or equivalent 5-year collaboration metrics. Control variables were standardized before inclusion in the model.

## S4 Co-disciplinary Awards Analysis

### S4.1 Data Description

For computer science, we collected 7,971 awards given by the Institute of Electrical and Electronics Engineers (IEEE) and the Association for Computing Machinery (ACM) since 1966. For physics, we collected 17,904 awards, the majority of them from the American Physical Society (APS), with some from the Institute of Physics (IOP), Optica, the American Vacuum Society (AVS), and the Acoustical Society of America (ASA), since 1921. For chemistry, we gathered 3,277 awards given by the American Chemical Society (ACS) and the Royal Society of Chemistry (RCS) since 1869. Finally, we gathered 527 American Mathematics Society (AMS) awards given out since 1925. The dataset consists of five fields: award name, awardee name, year, awarding organization, and contribution (when available). The awards were scraped from official websites or from Wikipedia. We used GPT-4o to supplement the contribution information for ACS and RCS awards, which usually did not list the contribution of the authors.

### S4.2 Data Annotation Prompt with GFT-4o

We used the GPT-4o API to conduct this inference for each prize, using a specific snapshot for reproducibility. GPT-4o is a very large flagship model from OpenAI that performs exceptionally well on text evaluation tasks compared to existing models, rendering it suitable for our task. We prompted it with the below few-shot prompt

template for each award, where primary field is the awarding organization’s field and secondary field is the field being considered for pair work:

*I’m going to give you the name of a [primary field] award, the organization that awarded it, the person who received the award, and the year it was awarded, along with the stated context for the award if possible. All of this information will be factual. You have to consider all this information and your own knowledge to tell me if that researcher collaborated with [secondary field researchers], contributed to the use of [secondary field] methods in [primary field] or [primary field] methods in [secondary field] with their research based on what you know. You must answer with either ‘yes’ or ‘no’, with no other text of any kind.*

*Input structure: [year], [award name], [awarding organization], [awardee name], [reason (optional)] Your output: [yes or no]*

*\*\* Here are some examples: Input: [Example 1] Expected output: [yes/no]*

*Input: [Example 2] Expected output: [yes/no]*

*Input: [Example 3] Expected output: [yes/no]*

*Input: [Example 4] Expected output: [yes/no] \*\**

*Let us begin. Input: [input]*

The above prompt template was used for each pair of fields we considered with slight manual adjustments to wording when necessary to improve prompt comprehension. The pairs that were compared were Physics-CS, Physics-Chemistry, Physics-Math, CS-Physics, CS-Chemistry, CS-Math, Chemistry-CS and Math-CS with the first field in each pair being the primary field. Figure S3 compares CS-to-secondary field co-disciplinary prizes with Physics-to-secondary field co-disciplinary prizes.

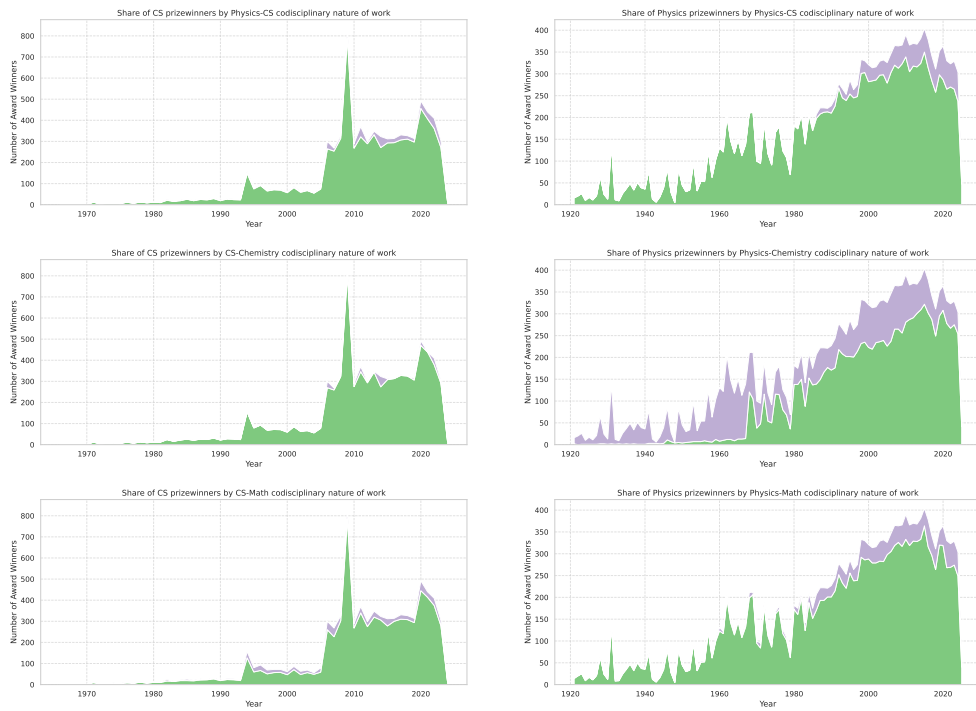

**Fig. S3:** Comparison of Computer Science prizes and Physics prizes by share of co-disciplinary awards between various fields each year. Green shade indicates in-discipline awards and purple shade indicates co-disciplinary awards.
